# Supplementary material for: Long-time memory effects in a localizable central spin problem
Source: arXiv:2105.04561 source file (2022-01-18)
Supplement: Supplementary file 1 [file supplement.pdf]

# Supplemental Material for "Long-time memory effects in a localizable central spin problem"

This supplement is divided as follows:

SM I: We provide details on the calculation for the short time $\propto t^2$ decay of the memory kernel.

SM II: We compare the intermediate time behaviors for disorder distributions different from the one shown in the main text, which was box-distributed with $W = 6J$. Here we show results for $W = 0.5J$ and $W = 2J$, for which the bath is delocalized at all couplings due to low disorder, and we additionally show the case of Gaussian distributed disorder.

SM III: We show additional numerics for the case of Gaussian distributed disorder, with variance matching that of the box-distributed disorder in the main text.

SM IV: We compare the integrated memory kernel $\kappa(t)$ between the interacting ($J = 1$) and noninteracting ($J = 0$) cases, for box distributed disorder $W = 6$ and Gaussian distributed disorder with $W = 6$.

SM V: We analyze the long-time behavior of the memory kernel, focusing on: 1) the long-time tail for a bath initially at infinite temperature, which we argue produces a power-law decay with a different exponent than what we found numerically in the main text; and 2) an analysis of the bias introduced by averaging over only a finite number of disorder realizations.

SM VI: We specify the finite-difference and quadrature schemes we employed to solve for the memory kernel.

SM VII: We provide a short discussion on the connection of the scalar memory kernel we chose to work with in the main text to the more common matrix memory kernel.

SM VIII: We discuss the appearance of off-axis poles in the Laplace-transform of the memory kernel for a single disorder realization, and show simple examples to establish that these poles–which give rise to unbounded exponential growth–are associated with exceptional points of the projected Liouvillian. By sampling real $3\times 3$ Hamiltonians, we provide further indication that these off-axis poles are suppressed when the eigenstates of the coupled problem remain "close" to the eigenstates of the uncoupled problem.

## I. SHORT TIME BEHAVIOR OF THE MEMORY KERNEL

In this section we reproduce the calculation for the short time behavior of the scalar memory kernel $K(t)$. The zeroth and second derivatives of $K(t)$ at $t = 0$ are given respectively by

$$K(t=0) = -p_0^{(2)}(t=0) \tag{1}$$

$$K^{(2)}(t=0) = -p_0^{(4)}(t=0) + \left(p_0^{(2)}(t=0)\right)^2 . \tag{2}$$

For a single realization of disorder, we therefore need

$$p_0^{(2)}(t=0) = -\operatorname{Tr}\left((|0\rangle\langle 0| \otimes \hat{I}_B)\,[H,[H,|0\rangle\langle 0| \otimes \rho_B]]\right)$$

$$p_0^{(4)}(t=0) = \operatorname{Tr}\left((|0\rangle\langle 0| \otimes \hat{I}_B)\,[H,[H,[H,[H,|0\rangle\langle 0| \otimes \rho_B]]]]\right).$$

Throughout the calculation we shall rely on the Pauli algebra,

$$\left[\hat{\sigma}^z, \hat{\sigma}^\pm\right] = \pm 2\hat{\sigma}^\pm \quad \left[\hat{\sigma}^+, \hat{\sigma}^-\right] = \hat{\sigma}^z \quad \left\{\hat{\sigma}^z, \hat{\sigma}^\pm\right\} = 0 \quad \left\{\hat{\sigma}^+, \hat{\sigma}^-\right\} = \hat{I},$$

along with the commutator identity for operators $A_i$ that commute with $B_i$ but not within each group,

$$[A_1B_1, A_2B_2] = [A_1, A_2]\, B_1B_2 + A_2A_1\,[B_1, B_2] \tag{3}$$

$$= [A_1, A_2]\,\frac{\{B_1, B_2\}}{2} + \frac{\{A_2, A_1\}}{2}\,[B_1, B_2]\,. \tag{4}$$

We shall also make use of the following identity to reduce the number of nested commutators:

$$\mathrm{Tr}\left(A\left[B,C\right]\right)=-\,\mathrm{Tr}\left(\left[B,A\right]C\right).$$

In the following we shall assume that $[\sum_i \hat{\sigma}_i^z, \rho_B] = [\sum_i \hat{\sigma}_i^z, H_B] = 0$. The first commutators can be reduced to

$$\begin{aligned}
\Big[H, |0\rangle\langle 0| \otimes \hat{I}_B\Big] &= \cancelto{0}{\Big[H_S, |0\rangle\langle 0| \otimes \hat{I}_B\Big]} + \cancelto{0}{\Big[H_B, |0\rangle\langle 0| \otimes \hat{I}_B\Big]} + \Big[V, |0\rangle\langle 0| \otimes \hat{I}_B\Big] \\
&= \gamma_\perp \sum_{i=1}^{L} \sum_{\pm} \Big[\hat{\tau}^{\pm}\hat{\sigma}_i^{\mp}, |0\rangle\langle 0| \otimes \hat{I}_B\Big] + \gamma_z \sum_{i=1}^{L} \cancelto{0}{\Big[\hat{\tau}^{z}\hat{\sigma}_i^{z}, |0\rangle\langle 0| \otimes \hat{I}_B\Big]} \\
&= \gamma_\perp \sum_{i=1}^{L} |1\rangle\langle 0| \otimes \hat{\sigma}_i^- - |0\rangle\langle 1| \otimes \hat{\sigma}_i^+ \\
[H, |0\rangle\langle 0| \otimes \hat{\rho}_B] &= \cancelto{0}{[H_S, |0\rangle\langle 0| \otimes \hat{\rho}_B]} + [H_B, |0\rangle\langle 0| \otimes \hat{\rho}_B] + [V, |0\rangle\langle 0| \otimes \hat{\rho}_B] \\
&= |0\rangle\langle 0| \otimes [H_B, \hat{\rho}_B] + \gamma_\perp \sum_{i=1}^{L} \sum_{\pm} \Big[\hat{\tau}^{\pm}\hat{\sigma}_i^{\mp}, |0\rangle\langle 0| \otimes \hat{\rho}_B\Big] + \gamma_z \cancelto{0}{\left[\hat{\tau}^z \otimes \left(\sum_{i=1}^{L} \hat{\sigma}_i^z\right), |0\rangle\langle 0| \otimes \hat{\rho}_B\right]} \\
&= |0\rangle\langle 0| \otimes [H_B, \hat{\rho}_B] + \gamma_\perp \sum_{i=1}^{L} |1\rangle\langle 0| \otimes \left(\hat{\sigma}_i^- \hat{\rho}_B\right) - |0\rangle\langle 1| \otimes \left(\hat{\rho}_B \hat{\sigma}_i^+\right).
\end{aligned}$$

These two expressions allow us to immediately evaluate $p_0^{(2)}(t=0)$, giving

$$\begin{aligned}
-p_0^{(2)}(t=0) &= \gamma_\perp \,\mathrm{Tr}\left\{\left(\sum_{j=1}^{L} |0\rangle\langle 1| \otimes \hat{\sigma}_j^+ - |1\rangle\langle 0| \otimes \hat{\sigma}_j^-\right)\left(|0\rangle\langle 0| \otimes [H_B, \hat{\rho}_B] + \gamma_\perp \sum_{i=1}^{L} |1\rangle\langle 0| \otimes \left(\hat{\sigma}_i^- \hat{\rho}_B\right) - |0\rangle\langle 1| \otimes \left(\hat{\rho}_B \hat{\sigma}_i^+\right)\right)\right\} \\
&= \gamma_\perp^2 \sum_{i,j=1}^{L} \mathrm{Tr}\left\{\left(|0\rangle\langle 1| \otimes \hat{\sigma}_j^+ - |1\rangle\langle 0| \otimes \hat{\sigma}_j^-\right)\left(|1\rangle\langle 0| \otimes \left(\hat{\sigma}_i^- \hat{\rho}_B\right) - |0\rangle\langle 1| \otimes \left(\hat{\rho}_B \hat{\sigma}_i^+\right)\right)\right\} \\
&= \gamma_\perp^2 \sum_{i,j=1}^{L} \mathrm{Tr}\left(|0\rangle\langle 0| \otimes \left(\hat{\sigma}_j^+ \hat{\sigma}_i^- \hat{\rho}_B\right) + |1\rangle\langle 1| \otimes \left(\hat{\rho}_B \hat{\sigma}_i^+ \hat{\sigma}_j^-\right)\right) \\
&= \gamma_\perp^2 \sum_{i,j=1}^{L} \mathrm{Tr}_B\left(\left\{\hat{\sigma}_j^+, \hat{\sigma}_i^-\right\} \hat{\rho}_B\right) = \gamma_\perp^2 \sum_{i,j=1}^{L} \mathrm{Tr}_B\left(\left\{\hat{\sigma}_j^+, \hat{\sigma}_i^-\right\} \hat{\rho}_B\right) \\
&= L\gamma_\perp^2 + \gamma_\perp^2 \sum_{i\neq j}^{L} \mathrm{Tr}_B\left(\left\{\hat{\sigma}_j^+, \hat{\sigma}_i^-\right\} \hat{\rho}_B\right).
\end{aligned}$$

When the initial bath state has a single pattern of magnetization (i.e. it is a product state of $\hat{\sigma}_i^z$ eigenstates), the initial value of the memory kernel will be $K(t=0) = L\gamma_\perp^2$, independent of the disorder realization as well as intrabath interactions. The fact that $K^{(2)}(t=0)$ is linear in the disorder-dependent quantity $p_0^{(4)}(t=0)$, when combined with the disorder-independence of $p_0^{(2)}(t=0)$, implies at least at short times it does not matter when the disorder averaging is performed. That is, averaging $p_0$ before calculating $K(t)$ will give the same result as averaging over all $K(t)$ associated with each realization of $p_0$. This gives an explicit example of our claim that for short times $K_{\mathrm{avg}}(t) \approx \overline{K}(t)$.

Evaluation of the fourth derivative for $p_0$ is more involved, but proceeds along a similar route. Generally speaking, note that these derivatives rely on the dynamics of coherences (i.e. off-diagonal elements) in the full density matrix.

$$
\begin{aligned}
\left[H,\left[H,|0\rangle\langle 0|\otimes \hat{I}_B\right]\right] &= \gamma_\perp\left[H,\hat{\tau}^+\otimes\hat{M}_B^- - \hat{\tau}^-\otimes\hat{M}_B^+\right]\\
&= \gamma_\perp\left(\hat{\tau}^+\otimes\left[H_B,\hat{M}_B^-\right] - \hat{\tau}^-\otimes\left[H_B,\hat{M}_B^+\right]\right)\\
&\quad + \gamma_\perp\gamma_z\left(\hat{\tau}^+\otimes\left\{\hat{M}_B^z,\hat{M}_B^-\right\} + \hat{\tau}^-\otimes\left\{\hat{M}_B^z,\hat{M}_B^+\right\}\right)\\
&\quad + \gamma_\perp^2\left(|0\rangle\langle 0|\otimes\left(\hat{M}_B^+\hat{M}_B^- + \hat{M}_B^+\hat{M}_B^-\right) - |1\rangle\langle 1|\otimes\left(\hat{M}_B^-\hat{M}_B^+ + \hat{M}_B^-\hat{M}_B^+\right)\right)
\end{aligned}
$$

$$
\begin{aligned}
[H,[H,|0\rangle\langle 0|\otimes\hat{\rho}_B]] &= \left[H,|0\rangle\langle 0|\otimes[H_B,\hat{\rho}_B] + \gamma_\perp\left(\hat{\tau}^+\otimes\hat{M}_B^-\hat{\rho}_B - \hat{\tau}^-\otimes\hat{\rho}_B\hat{M}_B^+\right).\right]\\
&= |0\rangle\langle 0|\otimes[H_B,[H_B,\hat{\rho}_B]]\\
&\quad + \gamma_\perp\left(\hat{\tau}^+\otimes\left[H_B,\hat{M}_B^-\hat{\rho}_B\right] - \hat{\tau}^-\otimes\left[H_B,\hat{\rho}_B\hat{M}_B^+\right]\right)\\
&\quad + \gamma_\perp\left(\hat{\tau}^+\otimes\hat{M}_B^-\left[H_B,\hat{\rho}_B\right] - \hat{\tau}^-\otimes\left[H_B,\hat{\rho}_B\right]\hat{M}_B^+\right)\\
&\quad + \gamma_\perp\gamma_z\left(\hat{\tau}^z|0\rangle\langle 0|\otimes\cancelto{0}{\left[\hat{M}_B^z,[H_B,\hat{\rho}_B]\right]} + \hat{\tau}^+\otimes\left\{\hat{M}_B^z,\hat{M}_B^-\hat{\rho}_B\right\} + \hat{\tau}^-\otimes\left\{\hat{M}_B^z,\hat{\rho}_B\hat{M}_B^+\right\}\right)\\
&\quad + \gamma_\perp^2\left(|0\rangle\langle 0|\otimes\left(\hat{M}_B^+\hat{M}_B^-\hat{\rho}_B + \hat{\rho}_B\hat{M}_B^+\hat{M}_B^-\right) - |1\rangle\langle 1|\otimes\left(\hat{M}_B^-\hat{\rho}_B\hat{M}_B^+ + \hat{M}_B^-\hat{\rho}_B\hat{M}_B^+\right)\right)\\
&= |0\rangle\langle 0|\otimes[H_B,[H_B,\hat{\rho}_B]]\\
&\quad + \gamma_\perp\left(\hat{\tau}^+\otimes\left[H_B,\hat{M}_B^-\hat{\rho}_B\right] - \hat{\tau}^-\otimes\left[H_B,\hat{\rho}_B\hat{M}_B^+\right]\right)\\
&\quad + \gamma_\perp\left(\hat{\tau}^+\otimes\hat{M}_B^-\left[H_B,\hat{\rho}_B\right] - \hat{\tau}^-\otimes\left[H_B,\hat{\rho}_B\right]\hat{M}_B^+\right)\\
&\quad - 2\gamma_\perp\gamma_z\left(\hat{\tau}^+\otimes\hat{M}_B^-\hat{\rho}_B + \hat{\tau}^-\otimes\hat{\rho}_B\hat{M}_B^+\right)\\
&\quad + \gamma_\perp^2\left(|0\rangle\langle 0|\otimes\left(\hat{M}_B^+\hat{M}_B^-\hat{\rho}_B + \hat{\rho}_B\hat{M}_B^+\hat{M}_B^-\right) - |1\rangle\langle 1|\otimes\left(\hat{M}_B^-\hat{\rho}_B\hat{M}_B^+ + \hat{M}_B^-\hat{\rho}_B\hat{M}_B^+\right)\right)
\end{aligned}
$$

There will be 6 contributions to the trace:

1. $\gamma_\perp^2\,\mathrm{Tr}_B\left(\left(\hat{M}_B^z\hat{M}_B^- + \hat{M}_B^+\hat{M}_B^z\right)[H_B,[H_B,\hat{\rho}_B]]\right) = 0$ since $\hat{M}_B^z\hat{\rho}_B = \hat{\rho}_B\hat{M}_B^z = 0$
2. $-\gamma_\perp^2\,\mathrm{Tr}_B\left(\left[H_B,\hat{M}_B^+\right]\left(\left[H_B,\hat{M}_B^-\hat{\rho}_B\right] + \hat{M}_B^-\left[H_B,\hat{\rho}_B\right]\right) + \left[H_B,\hat{M}_B^-\right]\left(\left[H_B,\hat{\rho}_B\hat{M}_B^+\right] + \left[H_B,\hat{\rho}_B\right]\hat{M}_B^+\right)\right)$
3. $\gamma_\perp^2\gamma_z\,\mathrm{Tr}_B\left(\left\{\hat{M}_B^z,\hat{M}_B^+\right\}\left(\left[H_B,\hat{M}_B^-\hat{\rho}_B\right] + \hat{M}_B^-\left[H_B,\hat{\rho}_B\right]\right) - \left\{\hat{M}_B^z,\hat{M}_B^-\right\}\left(\left[H_B,\hat{\rho}_B\hat{M}_B^+\right] + \left[H_B,\hat{\rho}_B\right]\hat{M}_B^+\right)\right)$
4. $-2\gamma_\perp^2\gamma_z\,\mathrm{Tr}_B\left(-\left[H_B,\hat{M}_B^+\right]\hat{M}_B^-\hat{\rho}_B + \left[H_B,\hat{M}_B^-\right]\hat{\rho}_B\hat{M}_B^+\right)$
5. $-2\gamma_\perp^2\gamma_z^2\,\mathrm{Tr}_B\left(\left\{\hat{M}_B^z,\hat{M}_B^-\right\}\hat{\rho}_B\hat{M}_B^+ + \left\{\hat{M}_B^z,\hat{M}_B^+\right\}\hat{M}_B^-\hat{\rho}_B\right) = 8\gamma_\perp^2\gamma_z^2\,\mathrm{Tr}_B\left(\hat{M}_B^+\hat{M}_B^-\hat{\rho}_B\right)$
6. $\gamma_\perp^4\,\mathrm{Tr}_B\left(\left\{\hat{M}_B^+,\hat{M}_B^-\right\}\left(\hat{M}_B^+\hat{M}_B^-\hat{\rho}_B + \hat{\rho}_B\hat{M}_B^+\hat{M}_B^- + 2\hat{M}_B^-\hat{\rho}_B\hat{M}_B^+\right)\right)$

The traces can be evaluated and disorder averaged in the Neel state to give

$$
p_0^{(4)} = \underbrace{L\gamma_\perp^2\left(\frac{W^2}{3} - 16J_z^2 - 4J_\perp^2 + 16J_\perp J_z\right)}_{\boxed{2}} + \underbrace{4L\gamma_\perp^2\gamma_z J_\perp}_{\boxed{3}} + \underbrace{2L\gamma_\perp^2\gamma_z(4J_z - J_\perp)}_{\boxed{4}} + \underbrace{4\gamma_\perp^2\gamma_z^2 L}_{\boxed{5}} + \underbrace{L\gamma_\perp^4(3L-4)}_{\boxed{6}}. \tag{5}
$$

Using the couplings for our model, the second derivative of the scalar memory kernel with an initial Neel bath state is given by

$$
K^{(2)}(t=0) = -\left(\frac{W^2}{3} + \frac{3}{4}\frac{\gamma}{L} + \frac{3}{4}\frac{\gamma^2}{L} - \frac{3}{4}\frac{\gamma^2}{L^2}\right) \tag{6}
$$

## II. INTERMEDIATE TIME BEHAVIOR FOR DIFFERENT DISORDER DISTRIBUTIONS

We show in Fig. 1 the (rescaled) memory kernel on intermediate times. In all four cases, the disorder distribution is held fixed as $\gamma$ changes. In the cases of box disorder, Fig. 1(a,c,d), the same patterns of $h_i$ scaled to the specified $W$ were used. For large values $W = 6$ when localization is expected, it can be seen in Fig. 1(a,b) that the same patterns of "shot noise" can be seen in the memory, even as $\gamma$ changes. This is the $\gamma$ insensitivity we argued for in the main text. In contrast, for the cases of weak disorder such that the bath is not localized it is evident that the $\gamma$ insensitive regime in $K_{\text{avg}}(t)$ is either absent or very quickly suppressed as $\gamma$ increases.

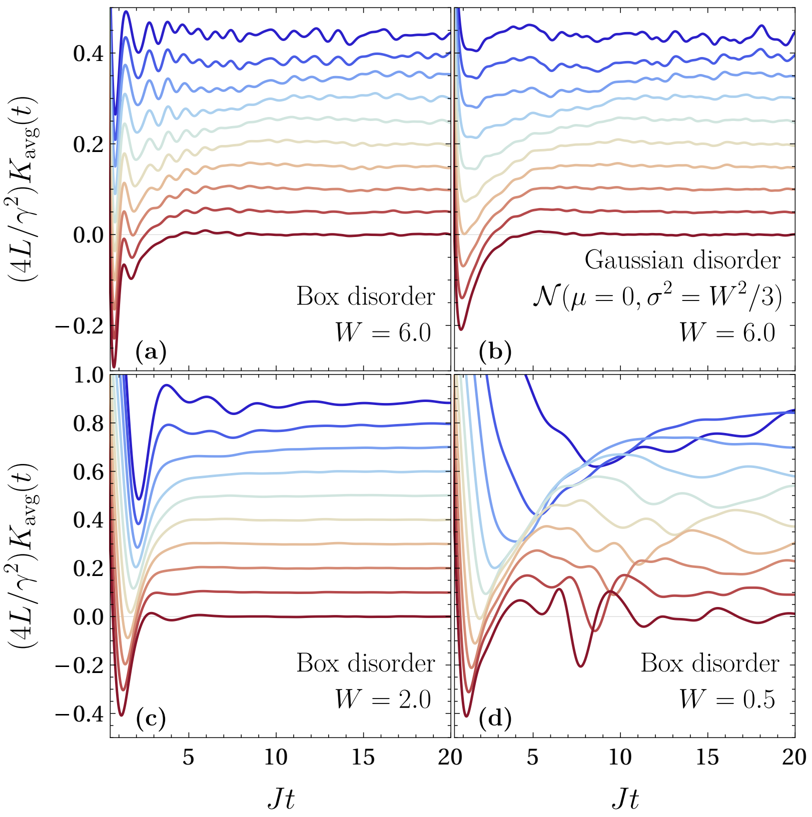


FIG. 1. Intermediate-time behavior of the memory kernel with $L = 12$, for different distributions of the random local fields $h_i$. Box disorder refers to $h_i \in [-W, W]$. The curves from top to bottom denote $\gamma = 1$(blue), $\cdots$, 10(red). For clarity, the data in **(a)** and **(b)** are shifted upwards in increments of 0.05, while the shift for **(c)** and **(d)** is in increments of 0.1.

## III. GAUSSIAN DISTRIBUTED DISORDER

In this section we show results for the same model, with $h_i$ drawn iid from Gaussian distributions with the same mean and variance as that of the box model, $h_i \sim \mathcal{N}(0, \sigma^2 = W^2/3)$.

At weak couplings when there should be localization, we see in Fig. 2 that the distribution of disorder indeed has a strong effect on the memory in the intermediate time regime, as we argued in the main text.

The importance of the disorder distribution on intermediate timescales is clearly seen from the integrated memory, $\kappa(t) \equiv \int_0^t K_{\text{avg}}(\tau)d\tau$, in Fig. 2b. This figure shows also why extrapolation of the populations may be more feasible to attempt for the thermalizing phase as opposed to the localized phase, at least on the fixed simulation time $Jt_{\max} = 100$.

The long-time behaviors of $K(t)$ are found to be qualitatively unchanged (see Fig. 3). There still exists exponential growth of the memory for certain realizations of disorder and the tail of $K_{\text{avg}}(t)$ is still consistent with a power-law decay, as seen through the application of the ansatz Eq. (**??**) of the main text.

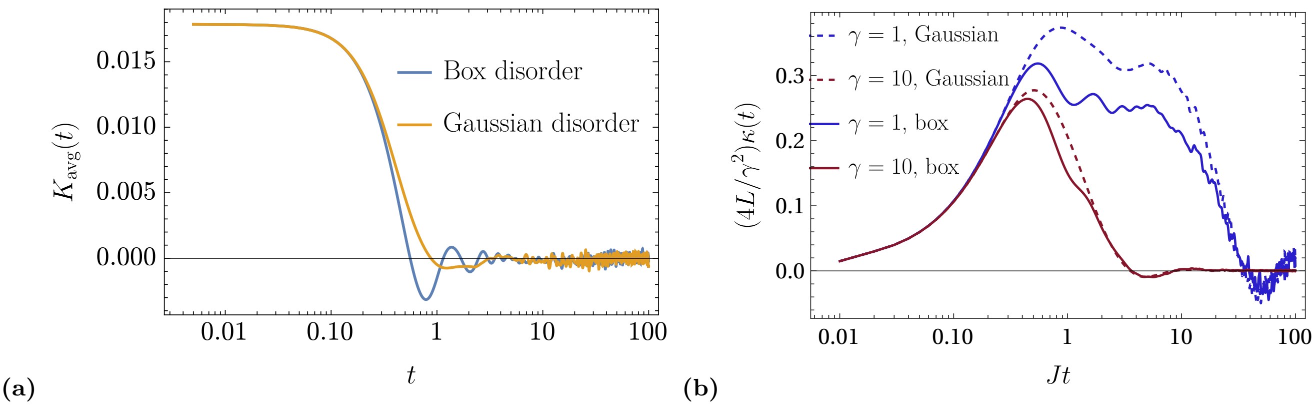


FIG. 2. **(a)** Memory kernel for the averaged population, $K_{\rm avg}(t)$ for $L = 14$ at $\gamma = 1$. The intermediate time oscillations found in the case of box-distributed disorder are absent in the Gaussian-distributed case. **(b)** Integrated memory kernel for the averaged population, $K_{\rm avg}(t)$ for $L = 14$ at $\gamma = 1$ (blue) and 10 (red), and for box (solid) and Gaussian (dashed) distributed disorder. The data shown is computed from 12800 realizations of disorder, except for the $\gamma = 1$ case with box disorder, which uses 1600 realizations.

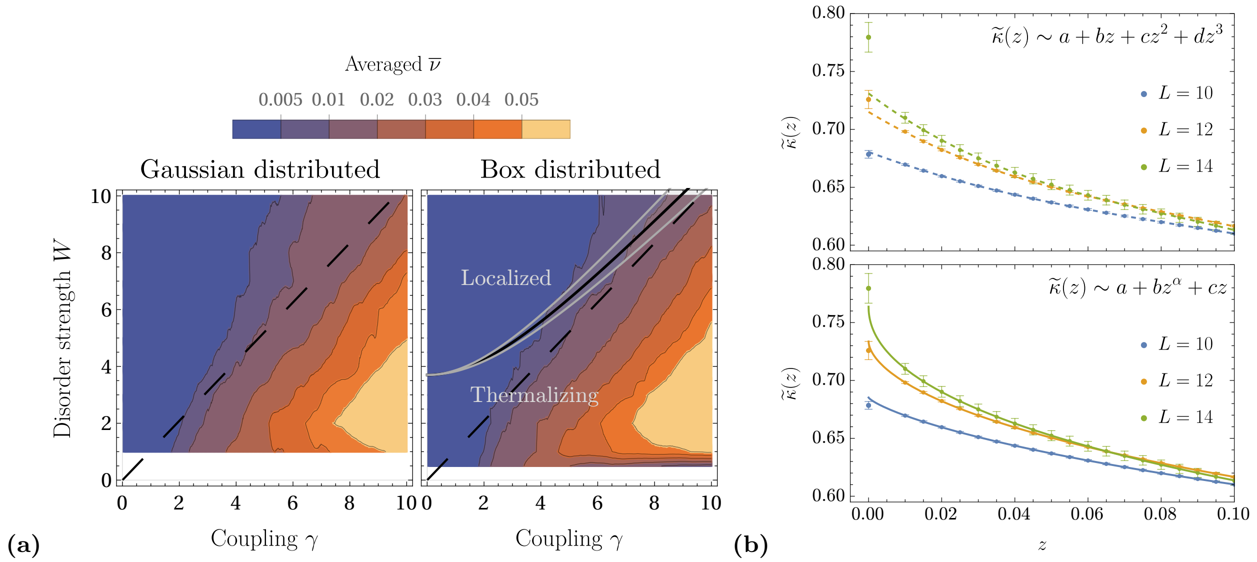


FIG. 3. Long-time behavior of the memory kernel for Gaussian distributed disorder. **(a)** Average rate of exponential growth for memory kernels in a single realization of disorder, where $L = 4$. The black dashed line in the Gaussian disorder case is the same as that for the box disorder, and is solely to help compare the two cases. **(b)** Extrapolation to $z = 0$ for the integrated memory kernel $\kappa(t)$, fitting to two ansatzes. Data points at $z = 0$ are independent calculations from exact diagonalization, while the data at $z > 0$ used for the fit are calculated using the Chebyshev polynomial method for time propagation.

## IV. EFFECT OF INTRABATH INTERACTIONS ON THE MEMORY KERNEL

In Fig. 4 we show the integral of the memory kernel $\kappa(t) = \int_0^t K_{\rm avg}(\tau)d\tau$. It is seen that the short time behaviors are largely the same between the interacting and noninteracting cases, for both box and Gaussian distributed disorder. For box disorder of $W = 6$ at strong coupling in the thermalized phase $\gamma = 10$, we observe a decaying oscillation on the timescales when, for $J = 1$, $\kappa(t)$ is decaying as a power law $\sim t^{-1-\zeta}$. These oscillations do not come from random noise over disorder realizations, and results in a robust signal between different $L$, with oscillation period that appears to scale with $L$ (see inset of Fig. 4a). A similar contribution to $\kappa(t)$ appears also for the case of Gaussian distributed disorder (Fig. 4b). While the form of the oscillations appears to differ between distributions, the envelope function appears to be similar. We are unable to precisely ascertain the form of the envelope, but note that it is consistent with $\kappa(t) \sim t^{-2}$, which we show in dashed orange lines in Fig. 4 using the same prefactor for all plots.

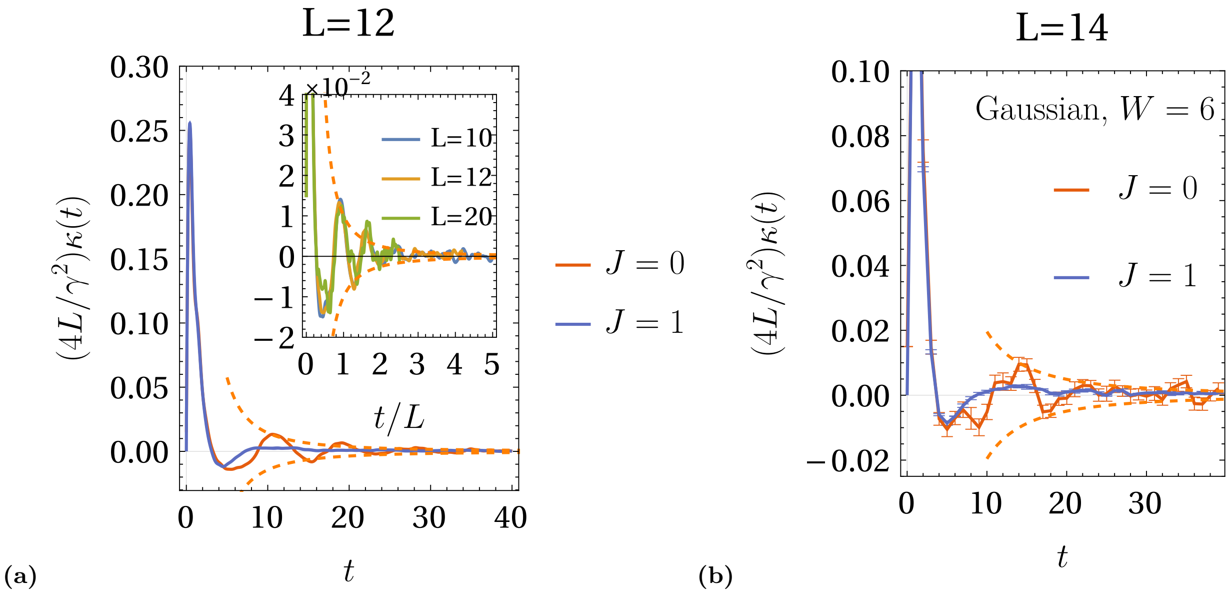


FIG. 4. Integral of the memory kernel between noninteracting ($J = 0$) and interacting ($J = 1$) cases, for **(a)** box distributed ($W = 6$) and **(b)** Gaussian distributed disorder. In both distributions, when $J = 0$ there appears an oscillatory component to $\kappa(t)$ with amplitude larger than that of the power-law decay found for the case of $J = 1$. **(a, inset)** Integrated memory for $L = 10, 12, 20$, rescaled to show a collapse of the oscillations when $t \to t/L$. In all the plots, the orange dashed line is given by $10^{-2}/t^2$.

## V. LONG-TIME BEHAVIOR OF THE MEMORY KERNEL

### A. Initially infinite temperature bath

We take the limit where the initial state has the bath at its infinite temperature state, i.e. $\hat{\rho}(0) = (|0\rangle\langle 0| \otimes \hat{I}_B)/\text{dim}\mathcal{H}_B$. In this case, the Laplace-transformed population is

$$\widetilde{p_0}(z) = 2\frac{1}{2(\text{dim}\mathcal{H}_B)}\sum_{E',E}\frac{\left|\left\langle E\middle||0\rangle\langle 0|\otimes \hat{I}_B\middle|E'\right\rangle\right|^2}{z + i(E-E')},$$

which is exactly the Laplace transform of an infinite-temperature autocorrelation function

$$p_0(t-t') = 2C(t-t') \equiv 2\,\text{Tr}\left\{\frac{1}{2(\text{dim}\mathcal{H}_B)}\hat{p}_0(t)\hat{p}_0(t')\right\}.$$

We begin by assuming that the Hamiltonian is quantum chaotic at large couplings. After accounting for the symmetries present in the model, the spectrum of the Hamiltonian is assumed to follow the Wigner-Dyson distribution due to time-reversal invariance, and the eigenvectors appear like random vectors with respect to the product basis $\{|0\rangle, |1\rangle\} \otimes \{|\uparrow\rangle, |\downarrow\rangle\}^L$. The small $z$ limit of $\widetilde{p_0}(z)$ is dominated by the statistics of small energy differences $E - E'$. This is because away from the edges of the energy spectrum, the matrix element of the local observable $\hat{p}_0$ should be constant in accordance with the random matrix assumption, i.e.

$$\left|\left\langle E\middle||0\rangle\langle 0|\otimes \hat{I}_B\middle|E'\right\rangle\right|^2 \sim O\left(\frac{1}{4(\text{dim}\mathcal{H}_B)}\right).$$

This assumption breaks down at large energy differences, so we expect that our calculation will only qualitatively

reproduce the long-time behavior.

$$\begin{aligned}
\widetilde{p_0}(z) &\sim \frac{\text{constant}}{z} + \left(\frac{1}{2(\dim\mathcal{H}_B)}\right)^2 \sum_{E'\neq E} \frac{1}{z+i(E-E')} \\
&= \frac{\text{constant}}{z} + \frac{1}{2}\left(\frac{1}{2(\dim\mathcal{H}_B)}\right)^2 \sum_{E'\neq E} \frac{2z}{z^2+(E-E')^2} \\
&= \frac{\text{constant}}{z} + \frac{1}{2}\left(\frac{1/\langle\Delta E\rangle}{2(\dim\mathcal{H}_B)}\right) \int d\omega \frac{2z}{z^2+\omega^2} \underbrace{\sum_{E'\neq E}\left(\frac{1}{2(\dim\mathcal{H}_B)}\right)\delta\left[\frac{\omega-(E-E')}{\langle\Delta E\rangle}\right]}_{\equiv R_2(\omega/\langle\Delta E\rangle)}.
\end{aligned}$$

Here, $R_2(\varepsilon)$ denotes the (unfolded) pair correlation function for the Gaussian orthogonal ensemble (GOE). The constant must equal 1/2 by inspection, it being the final value of $p_0(t\to\infty)$. To estimate the small $z$ behavior of $\widetilde{p_0}(z)$, note that it will be largely determined by the behavior of $R_2(\omega/\langle\Delta E\rangle)$ for small $\omega$. It is well known that the small $\varepsilon$ behavior of $R_2(\varepsilon)$ is linear for GOE random matrices [1], from which we obtain the leading-order contribution to $\widetilde{p_0}(z) \sim z\log z$. This translates to the time-domain as a $t^{-2}$ decay. Thus we conclude that, if the Hamiltonian at strong couplings obeys random matrix theory, then the population dynamics with a bath at infinite temperature will relax as a power-law at long times.

### B. Bias from finite realizations of disorder

One must take care in attempting to extrapolate to infinite times using only finite-time information on the memory kernel. As we argued in the main text, there appears a small contribution to $K(t)$ decaying much more slowly compared to the transient behavior on timescales $Jt \lesssim 10$. At the same time, we note that the tail of $K(t)$ exhibits fluctuations between different samples of the disorder in the bath which, although decreasing in magnitude with increasing bath size, will still have nonnegligible influence on long-time extrapolations.

For $N_s$ samples of the disorder, we can average these to obtain an estimate of the averaged population and its associated memory kernel,

$$\begin{aligned}
p_0(t;N_s) &= \frac{1}{N_s}\sum_{i=1}^{N_s} p_0^{(i)}(t) \\
\frac{d}{dt}p_0(t;N_s) &= -\int_0^t d\tau\ K(t-\tau;N_s)p_0(\tau;N_s).
\end{aligned}$$

With these definitions, we therefore can identify

$$\begin{aligned}
\overline{p_0}(t) &\equiv \lim_{N_s\to\infty} p_0(t;N_s) & K_{\text{avg}}(t) &\equiv \lim_{N_s\to\infty} K(t;N_s) \\
&\equiv \overline{p_0(t;N_s)}, \qquad \forall N_s & &\neq \overline{K(t;N_s)} \qquad (!)
\end{aligned}$$

While the quantities on the right hands sides of the top lines are what we would like calculate, in practice we are only able to approximate the quantities in the bottom lines. Particularly, approximating $K_{\text{avg}}(t)$ using $\overline{K(t;N_s)}$ will introduce a bias that cannot be removed unless one takes the $N_s\to\infty$ limit. We can more formally analyze this approximation in Laplace space, where we have

$$\begin{aligned}
\widetilde{K}_{\text{avg}}(z) &= -z + \left(\overline{\widetilde{p_0}(z;N_s)}\right)^{-1} \\
\overline{\widetilde{K}(z;N_s)} &= -z + \overline{\left(\widetilde{p_0}(z;N_s)\right)^{-1}}.
\end{aligned}$$

Note that the Laplace transform of $p_0(t;N_s)$ is positive for nonnegative $z$. Since $1/x$ is a convex function, these

memory kernels can be related via Jensen's inequality,

$$\widetilde{K}_{\text{avg}}(z) \leq \overline{\widetilde{K}(z;N_s)}$$
$$\Downarrow$$
$$\frac{1}{1+\widetilde{K}_{\text{avg}}(z)/z} \geq \frac{1}{1+\overline{\widetilde{K}(z;N_s)}/z}.$$

Thus taking the $z \to 0^+$ limit, one sees that the extrapolated infinite-time populations may be underestimated if one uses $\overline{K(t;N_s)}$. The source of this systematic bias is due to the fact that $K(t)$ is a nonlinear function of $p_0(t)$. We would therefore like to estimate the magnitude of the nonlinearity to see if it will contribute significantly to the extrapolation of the infinite-time populations. If we formally consider $K(t)$ to be a function of $p_0(t)$ and expand around the infinitely-averaged result $\overline{p_0}(t)$, we have

$$K(t_n;N_s) = K(t_n;\infty) + \sum_m \left(p_0(t_m;N_s) - \overline{p_0(t_m)}\right)\partial_m K(t_n;\infty) \tag{7}$$

$$+\frac{1}{2}\sum_{\ell m}\left(p_0(t_\ell;N_s) - \overline{p_0(t_\ell)}\right)\left(p_0(t_m;N_s) - \overline{p_0(t_m)}\right)\partial_\ell\partial_m K(t_n;\infty) + \ldots \tag{8}$$

For a finite number of samples, $\alpha N_s$ where $\alpha$ is a positive integer, notice that the zeroth and linear order corrections can be cancelled

$$\begin{aligned} K(t_n;\alpha N_s) - \frac{1}{\alpha}\sum_{i=1}^{\alpha} K^{(i)}(t_n;N_s) &= \frac{1}{2}\sum_{\ell m}\Bigg[\left(p_0(t_\ell;\alpha N_s) - \overline{p_0(t_\ell)}\right)\left(p_0(t_m;\alpha N_s) - \overline{p_0(t_m)}\right) \\ &\quad - \frac{1}{\alpha}\sum_{i=1}^{\alpha}\left(p_0^{(i)}(t_\ell;N_s) - \overline{p_0(t_\ell)}\right)\left(p_0^{(i)}(t_m;N_s) - \overline{p_0(t_m)}\right)\Bigg]\partial_\ell\partial_m K(t_n;\infty) + \ldots \\ &\equiv \delta K(t_n;\alpha N_s, N_s). \end{aligned}$$

We explicitly compare the magnitude of the relative correction $K(t_n;\alpha N_s, N_s)$ in Fig. 5.

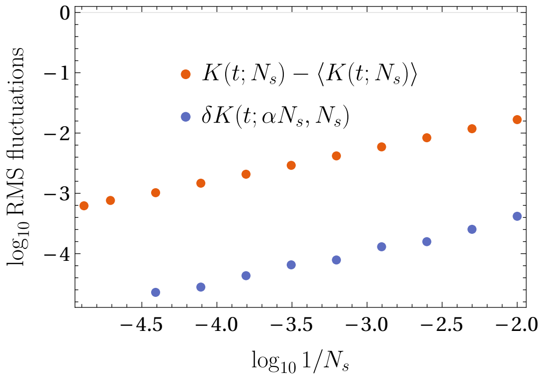


FIG. 5. Comparison between RMS fluctuations in the tail of $K(t)$ (orange dots) and RMS fluctuations in $K(t)$ resulting from bias introduced by a finite number of disorder realizations (blue dots). The system under consideration has $L = 12$ and $\gamma = 10$.

We see that the relative bias is over an order of magnitude smaller compared to the fluctuations in $K(t)$ contributed by the finite number of disorder realizations, which appear as the linear-in-$p_0$ correction in Eq. (7).

## VI. NUMERICAL INVERSION FOR MEMORY

Here we summarize the numerical method used to investigate the memory kernel without resorting to perturbation theory. For simplicity we shall restrict ourselves to the case of $H_S = 0$ with matrix memory kernels $\mathbb{K}$ and system propagators $\mathbb{U}_S$:

$$\frac{d}{dt}\mathbb{U}_S(t) = -\int_0^t dt'\,\mathbb{K}(t')\mathbb{U}_S(t-t').$$

We assume that the value of $\mathbb{K}(0)$ is known, a fact which allows us to use slightly higher order approximations. For a general bath state $\rho_B$, the initial value is $\gamma_\perp^2 \sum_{i,j,\pm} \mathrm{Tr}\left[\hat{\sigma}_i^\pm \hat{\sigma}_j^\mp \rho_B\right]$.

We discretize this equation as follows:

$$\dot{\mathbb{U}}_S(n\Delta t) = \frac{1}{\Delta t}\left(\frac{-\mathbb{U}_S((n-1)\Delta t)}{3} + \frac{-\mathbb{U}_S(n\Delta t)}{2} + \mathbb{U}_S((n+1)\Delta t) + \frac{-\mathbb{U}_S((n+2)\Delta t)}{6}\right) + O(\Delta t^3)$$

$$\int_0^{n\Delta t} dt' \mathbb{K}(t')\mathbb{U}_S(n\Delta t - t') = (\Delta t)\left(\frac{\mathbb{K}(0\Delta t)\mathbb{U}_S(n\Delta t) + \mathbb{K}(n\Delta t)\mathbb{U}_S(0\Delta t)}{2} + \sum_{m=1}^{n-1} \mathbb{K}(m\Delta t)\mathbb{U}_S((n-m)\Delta t)\right) + O(\Delta t^3).$$

The calculations in the main paper were performed with $J\Delta t = 0.01$ for $0 \leq Jt \leq 100$. By truncating the error terms and equating the two expressions, the memory kernel can be solved for via iterating back substitutions. We note that the numerically inverted solution displays spurious oscillations of period $2\Delta t$. This can be largely removed by taking the 2-element moving average, i.e.

$$\mathbb{K}\left((n+\frac{1}{2})\Delta t\right) = \frac{\mathbb{K}(n\Delta t) + \mathbb{K}((n+1)\Delta t)}{2}.$$

For example, in the case of a scalar memory kernel generating the dynamics such that $K(t) = \exp(-t/5)\cos(t)$, such an averaging procedure produces a much more well-behaved solution (see Figure 6).

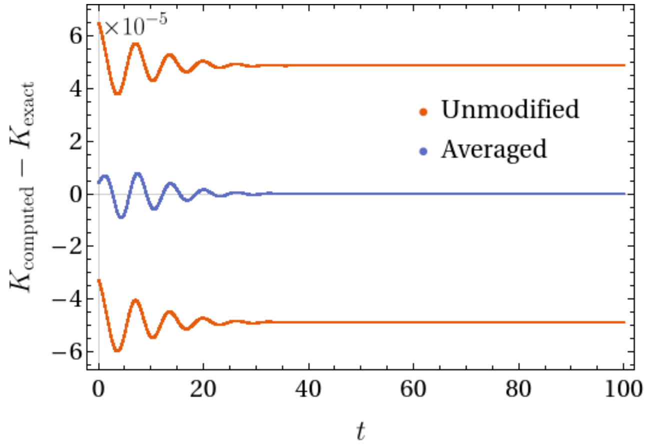


FIG. 6. Numerical inversion of dynamics generated by the memory kernel $K(t) = \exp(-t/5)\cos(t)$, compared against the exact solution. Without the 2-element moving average, the computed memory oscillates between the top and bottom bands on each timestep $\Delta t = 0.01$.

## VII. SCALAR MEMORY KERNEL

The derivation of the Nakajima-Zwanzig equation is agnostic with respect to choice of projection superoperators $\mathbb{P}$. Thus we have used this fact to our advantage in computing the memory kernel since projecting on to only a single distinguished variable, the $|0\rangle$ population,

$$\mathbb{P}_{\text{sca}}\hat{\rho} = (|0\rangle\langle 0| \otimes \hat{\rho}_B)\,\mathrm{Tr}\left\{(|0\rangle\langle 0| \otimes \hat{I}_B)\hat{\rho}\right\},$$

reduces the amount of independent trajectories required. This allows us to work with a scalar memory kernel, $K(t)$. We recognize that this is an unconventional choice of projector, with the usual choice being

$$\mathbb{P}_{\text{full}}\hat{\rho} = (\mathrm{Tr}_B\,\hat{\rho}) \otimes \hat{\rho}_B,$$

which gives rise to a tensor memory kernel $\mathbb{K}_{(mn),(ij)}$ describing how past values of the $(ij)$ element of the system's reduced density matrix $\hat{\rho}_S$ affect the $(mn)$ element of $\hat{\rho}_S$ at the current time.

The memory kernel in both cases follows the same form:

$$K(t) = \mathrm{Tr}\left[\mathbb{P}_{\mathrm{sca}}\mathbb{L}\mathbb{Q}_{\mathrm{sca}}\exp\left\{-i\mathbb{Q}_{\mathrm{sca}}\mathbb{L}\mathbb{Q}_{\mathrm{sca}}t\right\}\mathbb{Q}_{\mathrm{sca}}\mathbb{L}\mathbb{P}_{\mathrm{sca}}\right] \tag{9}$$

$$\mathbb{K}(t) = \mathrm{Tr}\left[\mathbb{P}_{\mathrm{full}}\mathbb{L}\mathbb{Q}_{\mathrm{full}}\exp\left\{-i\mathbb{Q}_{\mathrm{full}}\mathbb{L}\mathbb{Q}_{\mathrm{full}}t\right\}\mathbb{Q}_{\mathrm{full}}\mathbb{L}\mathbb{P}_{\mathrm{full}}\right]. \tag{10}$$

$$\dot{p}_0(t) = -\int_0^t d\tau\, K(t-\tau)p_0(\tau) \tag{11}$$

$$\dot{p}_0(t) = \int_0^t d\tau\, \mathbb{K}_{(11),(11)}(t-\tau) - \int_0^t d\tau\, \left[\mathbb{K}_{(00),(00)}(t-\tau) + \mathbb{K}_{(11),(11)}(t-\tau)\right] p_1(\tau). \tag{12}$$

The difference between these two expressions is that, in the former case where the scalar memory kernel is directly defined from a suitable projection operator, the state $|1\rangle$ in the central qubit is explicitly treated as part of the bath. In the second case where this was not done, the influence of the $|1\rangle$ state on the population of the $|0\rangle$ state manifests as an external fluctuating force, $\int_0^t \mathbb{K}_{(11),(11)}(\tau)d\tau$.

These two master equations can be shown to give the same dynamics since the memory kernels are related as,

$$K(t) = \int_0^t d\tau\, \mathbb{K}_{(00),(00)}(t-\tau)\dot{G}(\tau)$$

$$\dot{G}(t) = -\int_0^t d\tau\, \mathbb{K}_{(11),(11)}(t-\tau)G(\tau), \qquad G(0) = 1.$$

Such a relation follows from the fact that the projection superoperators $\mathbb{P}_{\mathrm{sca}}$ and $\mathbb{P}_{\mathrm{full}}$ share a common term [2].

We can quickly derive the memory kernel in the eigenbasis by virtue of its relation with the trajectory $p_0(t)$. In the following, we adopt the notation: $|\psi_0\rangle$ denotes the initial bath state; $|0, B\rangle$ denotes the factorized state where the system is in $|0\rangle$ and the bath is in $|B\rangle$; and $|E\rangle$ denotes the eigenstate of energy $E$ of the combined system and bath. The population, in the time and Laplace domains, is given by

$$\begin{aligned} p_0(t) &= \sum_B \left| \sum_E e^{-iEt} \langle 0, B|E\rangle \langle E|0, \psi_0\rangle \right|^2 \\ &= \sum_B \sum_{E,E'} e^{-i(E-E')t} \langle 0, \psi_0|E'\rangle \langle E'|0, B\rangle \langle 0, B|E\rangle \langle E|0, \psi_0\rangle \\ \widetilde{p_0}(z) &= \sum_{E,E'} \underbrace{\left( \sum_B \langle E'|0, B\rangle \langle 0, B|E\rangle \right)}_{\equiv C(E',E)} \frac{\langle 0, \psi_0|E'\rangle \langle E|0, \psi_0\rangle}{z + i(E-E')}. \end{aligned}$$

Since the memory kernel is defined as $K(z) = -z + p_0(z)^{-1}$, we therefore have, after using the fact that the inner products in the above expression are real,

$$K(z) = -z + \left( \sum_E \frac{C(E,E)\left|\langle E|0, \psi_0\rangle\right|^2}{z} + 2z \sum_{E'>E} C(E', E) \frac{\langle 0, \psi_0|E'\rangle \langle E|0, \psi_0\rangle}{z^2 + (E-E')^2} \right)^{-1}$$

## VIII. APPEARANCE OF COMPLEX POLES FOR THE SCALAR MEMORY KERNEL

To verify the exponential growth of $K(t)$ we observe from directly inverting the Nakajima-Zwanzig equation in the time domain, we solve for the poles of $\widetilde{K}(z)$ numerically using 4096 bits of precision. Diagonalization and root-finding are respectively provided by the `GenericLinearAlgebra.jl` and the `PolynomialRoots.jl` packages in Julia. The rapid growth of the Liouville space's dimensionality limits this approach to system sizes $L \leq 6$.

The scalar memory kernel in Laplace space has a very simple form,

$$K(z) = -z + \left( \frac{\overline{p_0}}{z} + \sum_{n=1}^{N} \frac{A_n z}{z^2 + \omega_n^2} \right)^{-1},$$

where $\overline{p}_0 > 0$ is the value that $p_0(t)$ either decays to or oscillates around as $t \to \infty$. The frequencies $\omega_n$ are given by the difference of the $n$th pair of energies of the full Hamiltonian, $\omega_n = E' - E$ such that $E' > E$. The initial value of $p_0(0) = 1$ sets a constraint that $\overline{p_0} + \sum_n A_n = 1$. The requirement that $0 \leq p_0 \leq 1$ gives the pair of sufficient conditions $\overline{p_0} + \sum_n |A_n| \leq 1$ and $0 \leq \overline{p_0} - \sum_n |A_n|$.

### A. Exceptional points

For the Hamiltonian Eq. (**??**) of the main text, we illustrate our claim that there can exist exceptional points in the projected Liouvillian, which can then give rise to exponentially divergent scalar memory kernels. For simplicity, we fix $L = 2$ and take the bath to have zero magnetization. This makes the Hilbert space three-dimensional, and the Liouville space is therefore nine-dimensional. We can then directly write the Liouvillian $\mathbb{L} = \left[\hat{H}, \cdots\right]$ and projector $\mathbb{P} = \left|\hat{\rho}(0)\right)\left(|0\rangle\langle 0| \otimes \hat{I}_B\right|$ in matrix form, and compute the left and right eigendecompositions of $\mathbb{QLQ}$. In Fig. 7a we show the (right) eigenvalue dynamics of $\mathbb{QLQ}$ as the central coupling $\gamma$ is tuned. The red dotted lines indicate the values of $\gamma$ for which the projected Liouvillian becomes degenerate; the enumeration of all such exceptional points is shown in Fig. 7b. These are computed from the roots of the characteristic polynomial [3]

$$g(\gamma) = \det \mathbf{S}(\gamma) = 0$$
$$\mathbf{S} = \begin{pmatrix} \mu_{2N-2} & \mu_{2N-3} & \cdots & \mu_{N-1} \\ \mu_{2N-3} & \mu_{2N-4} & \cdots & \vdots \\ \vdots & \vdots & \mu_2 & \mu_1 \\ \mu_{N-1} & \cdots & \mu_1 & 1 \end{pmatrix} \tag{13}$$
$$\mu_p(\gamma) = \sum_{i=1} (\hat{O}_i|\left(\mathbb{QL}(\gamma)\mathbb{Q}\right)^p|\hat{O}_i).$$

At one of these exceptional points, $\gamma = \gamma_c$ for example, it is evident from Fig. 7a that two eigenvalues have become exactly degenerate. In actuality, there is a *coalescence* of eigenvalues exactly at $\gamma_c$, which is when the left and right eigenvectors display self-orthogonality. This is explicitly demonstrated in Fig. 7c.

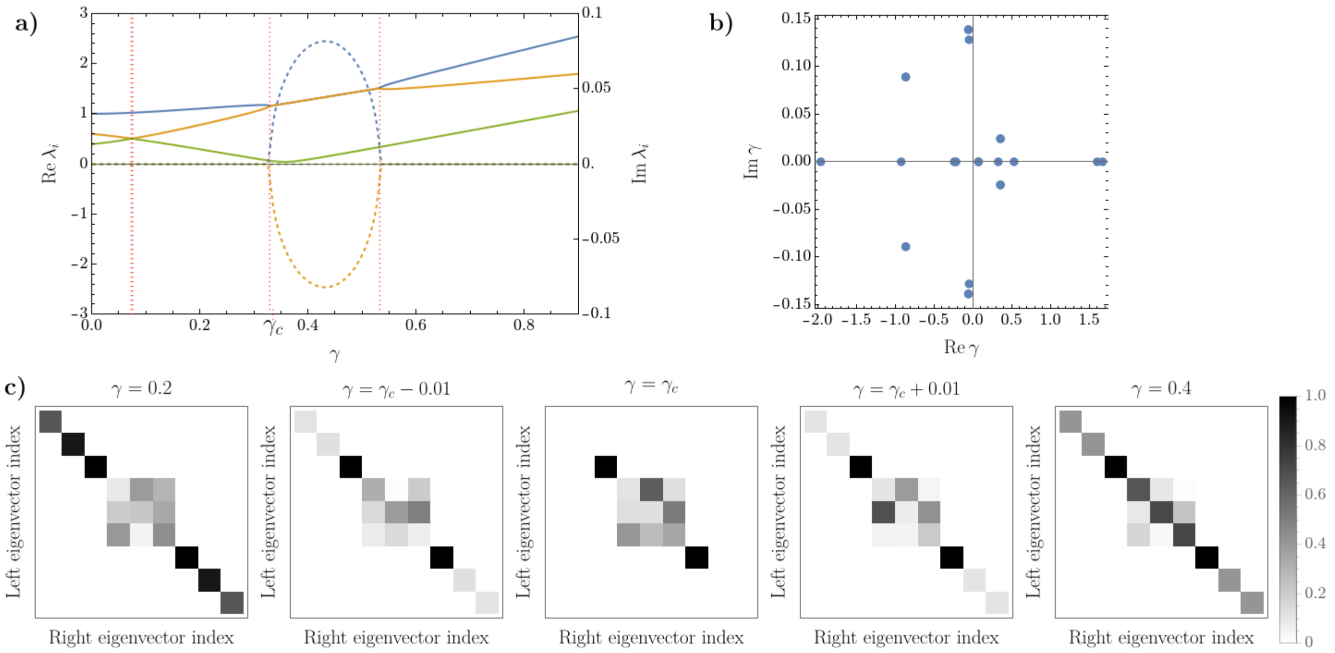


FIG. 7. Appearance of exceptional points in the projected Liouvillian $\mathbb{QLQ}$ for the model studied in the main text with a fixed disorder configuration and $L = 2$. **(a)** Right eigenvalues of $\mathbb{QLQ}$ as the central coupling $\gamma$ is increased. When $\gamma$ lies between two exceptional points on the branch singularity that connects them, the projected Liouvillian attains imaginary eigenvalues. **(b)** Exceptional points of $\mathbb{QL}(\gamma)\mathbb{Q}$ as obtained from Eq. (13). **(c)** Squared overlaps of the left and right eigenvectors of the projected Liouvillian. Exactly at the exceptional point labelled $\gamma_c$, it is seen that there are left and right eigenvectors that become orthogonal.

## B. Three eigenvalues

The system of three states is simplest one for analyzing the exponential growth in the scalar memory kernel, since it yields only three unique positive energy differences. This in turn leads to a cubic equation $f_3(x)$ for the poles of the memory kernel, and the roots of cubic equations are well characterized by the sign of the discriminant. WLOG, we define $\omega_1 = \Omega$, $\omega_2 = \delta$, and $\omega_3 = \Omega + \delta$, and the ratio of adjacent energy differences $r \equiv \delta/\Omega$. Since the physics should be invariant with respect to swapping $\Omega$ and $\delta$, we shall limit our discussion of $r$ on the restricted domain $[0, 1]$.

$$
\begin{aligned}
f_3(z^2) = (z^2)^3 &+ \underbrace{\left((1-A_1)\omega_1^2 + (1-A_2)\omega_2^2 + (1-A_3)\omega_3^2\right)}_{\equiv b}(z^2)^2 \\
&+ \underbrace{\left((\overline{p_0}+A_1)\omega_2^2\omega_3^2 + (\overline{p_0}+A_2)\omega_1^2\omega_3^2 + (\overline{p_0}+A_3)\omega_1^2\omega_2^2\right)}_{\equiv c}(z^2)^1 \\
&+ \underbrace{\overline{p_0}\omega_1^2\omega_2^2\omega_3^2}_{\equiv d}
\end{aligned}
$$

This is a real cubic polynomial in the variable $x \equiv z^2$. The properties of its zeroes are communicated through the sign of its discriminant $\Delta$, which for a general cubic equation $ax^3 + bx^2 + cx + d$ is given by

$$\Delta = b^2c^2 - 4ac^3 - 4b^3d - 27a^2d^2 + 18abcd.$$

When this quantity is negative, the equation will have two complex roots. Similarly, if $\Delta > 0$ and the coefficients of $f_3$ are strictly positive, there must be three real, negative roots. Assuming that $\overline{p_0} > 0$ implies $d > 0$. We can therefore work with a modified discriminant by dividing through by $d^2$, while retaining the properties of the original discriminant. Doing so results in

$$
\begin{aligned}
\Delta' &= \beta^2\gamma^2 + 18\beta\gamma - 4\gamma^3 - 4\beta^3 - 27 \\
\beta &= b/d^{1/3} \\
\gamma &= \gamma/d^{2/3}
\end{aligned}
$$

In terms of the ratio $r$, we have

$$
\begin{aligned}
\beta &= \frac{1}{\overline{p_0}^{1/3}}\left((1-A_1)r^{-2/3}(1+r)^{-2/3} + (1-A_2)r^{4/3}(1+r)^{-2/3} + (1-A_3)r^{-2/3}(1+r)^{4/3}\right) \\
\gamma &= \frac{1}{\overline{p_0}^{2/3}}\left((\overline{p_0}+A_1)r^{2/3}(1+r)^{2/3} + (\overline{p_0}+A_2)r^{-4/3}(1+r)^{2/3} + (\overline{p_0}+A_3)r^{2/3}(1+r)^{-4/3}\right)
\end{aligned}
$$

We find that the sufficient conditions provided by the bounds $0 \le p_0 \le 1 \Longrightarrow \overline{p_0} + \sum_n |A_n| \le 1$ and $0 \le \overline{p_0} - \sum_n |A_n|$ is too strict and evidently produces no complex poles. Instead, we shall randomly sample the $A_n$'s and $\overline{p_0}$.

In this three-state case, we parametrize the eigenstates using the axis-angle representation, where for the $k$th eigenstate ($k = 1, 2, 3$),

$$\left(\mathbf{v}^{(k)}\right)_j = \left(e^{-i\theta(\hat{\mathbf{S}}\cdot\mathbf{n})}\right)_{j,k},$$

where the unit vector $\mathbf{n}$ is defined by the polar angle $\psi$ and the aximuthal angle $\phi$. In terms of these three parameters, we define probabiility distribution as

$$P(\phi,\psi,\theta)\,d\phi\,d\psi\,d\theta = \frac{\sin\psi}{4\pi}\frac{1-\cos\theta}{\theta_{\max} - \sin\theta_{\max}}d\phi\,d\psi\,d\theta,$$

on the domain $0 \le \phi < 2\pi$, $0 \le \psi \le \pi$, and $0 \le \theta \le \theta_{\max}$, where $0 \le \theta_{\max} \le \pi$. As seen in Fig. 8, the angle $\theta_{\max}$ measures the maximum deviation between the eigenvectors and the system=bath decoupled basis states. This measure coincides with the Haar measure for the $3 \times 3$ circular orthogonal ensemble When $\theta_{\max} = \pi$. In the main text, we measure this deviation in terms of the minimum fidelity

$$f \equiv \cos\theta_{\max}.$$

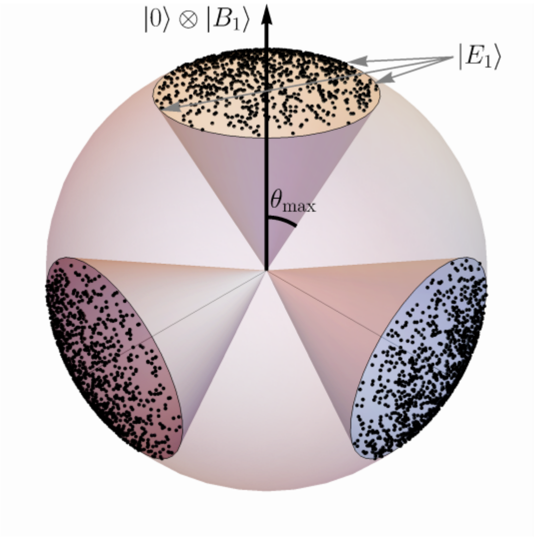


FIG. 8. Relationship between the system-bath decoupled basis (unit vectors on the $x, y, z$ axes) and the randomly sampled eigenvectors (black dots). The parameter $\theta_{\mathrm{max}}$ controls the maximum deviation of the eigenvectors from the basis (shaded regions bounded by cones).

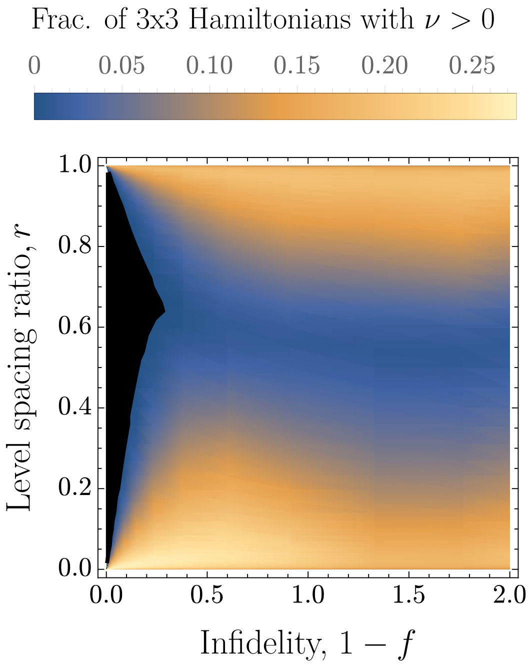


FIG. 9. Fraction of random real $3 \times 3$ Hamiltonians which show nonzero $\nu$. The fidelity $f \in [-1, 1]$ quantifies the minimum overlap between the eigenstates with the system-bath decoupled basis, with $f = 1$ when they coincide (see main text and supplement for details). Black regions indicate a fraction of exactly zero within the $10^7$ random configurations of eigenvectors sampled. The level spacing ratio is defined as $r \equiv \min(E_2 - E_1, E_3 - E_2)/\max(E_2 - E_1, E_3 - E_2)$ where $E_1 < E_2 < E_3$.

Consider a three-level system with nondengenerate eigenvalues $0 = E_1 < E_2 < E_3$. Since the overall scale of the energies does not matter, we can condense these into one parameter given by the level spacing ratio

$$r = \frac{\min(E_2 - E_1, E_3 - E_2)}{\max(E_2 - E_1, E_3 - E_2)}. \tag{14}$$

By fixing the energies we can sample random real Hamiltonians by generating random orthogonal matrices, whose columns constitute the eigenstates. To make connection with the reduced dynamics we consider in this paper, we

generate these eigenstates in the system-bath decoupled basis, $|0\rangle \otimes |B_{1\mathrm{or}2}\rangle$ and $|1\rangle \otimes |B_3\rangle$. A linear combination of the basis states occupying $|0\rangle$ forms the initial state $\hat{\rho}(0)$. We quantify the relationship between the random eigenstates $|E_i\rangle$ and the decoupled basis $|SB_n\rangle$ through the fidelity,

$$F(E_1, E_2, E_3) = \min_{n=1,2,3} \max_{i=1,2,3} \langle E_i|SB_n\rangle, \tag{15}$$

and uniformly sample $|E_i\rangle$ to satisfy the constraint $F(E_1, E_2, E_3) \geq f$. The minimum fidelity $f$ takes values between $-1$ and 1. In Fig. 9 we show the maximum infidelity $1 - f$, which intuitively should play a similar role to the system bath coupling $\gamma$ when both $1 - f$ and $\gamma$ are small.

For each pair of $(f, r)$ we can estimate the fraction of Hamiltonians and bath states–sampled uniformly subject to the constraint–that exhibit a nonzero $\nu$. This result is shown in Fig. 9. Exponential growth is seen to be prevalent near $r = 0$, which is when two eigenvalues of the Liouvillian become close to each other. This may be unsurprising given that exceptional points occur near level-crossings. More puzzling is the increasing prevalence of exponential growth as the level spacings become more uniform, i.e. as $r \to 1$. Finally, we observe zero instances of finite $\nu$ over $10^7$ random samples of $|E_i\rangle$ inside a contiguous region beginning around $F \gtrsim 0.6$ (black region in Fig. 9).


[1] H.-J. Stöckmann, Random matrices, in Quantum Chaos: An Introduction (Cambridge University Press, 1999) p. 59–134.
[2] N. Ng, D. T. Limmer, and E. Rabani, Note: Nonuniqueness of generalized quantum master equations for a single observable (2021), arXiv:2108.10937.
[3] M. Zirnbauer, J. Verbaarschot, and H. Weidenmüller, Destruction of order in nuclear spectra by a residual goe interaction, Nuclear Physics A **411**, 161 (1983).
